# Supplementary material for: A Large Scale Analysis of Android-Web Hybridization
Source: arXiv:2008.01725 source file (2020-08-05)
Supplement: Supplementary file 1 [file appendix-js-malware.tex]

\begin{table*}[h]
    \centering
        \begin{tabular}{p{15cm}c}
        \toprule
        \textbf{Program Fragment} & \textbf{\%age of Apps} \\
        \midrule
{\begin{lstlisting}[language=JavaScript,frame=none,aboveskip=0mm,belowskip=0mm,numbers=none]
javascript:window.HTMLOUT.processHTML(document.getElementById('SearchResults').innerHTML);
\end{lstlisting}} & 72.73 \\ \hline
{\begin{lstlisting}[language=JavaScript,frame=none,aboveskip=0mm,belowskip=0mm,numbers=none]
(function() {var flurryBridgeCtor=function(w) {
    var flurryadapter={};flurryadapter.flurryCallQueue=[];
    flurryadapter.flurryCallInProgress=false;
    flurryadapter.callComplete=function(cmd){
        if(this.flurryCallQueue.length==0){
            this.flurryCallInProgress=false;return
        }
        var adapterCall=this.flurryCallQueue.splice(0,1)[0];this.executeNativeCall(adapterCall);
        return\interstitial
    }
}
\end{lstlisting}} & 7.44 \\ \hline
{\begin{lstlisting}[language=JavaScript,frame=none,aboveskip=0mm,belowskip=0mm,numbers=none,breaklines=true]
(function () { var flurryBridgeCtor = function (w) {
var flurryadapter = {}; flurryadapter.flurryCallQueue = []; flurryadapter.flurryCallInProgress = false; flurryadapter.callComplete = function (cmd) { if (this.flurryCallQueue.length == 0) { this.flurryCallInProgress = false; return } var adapterCall = this.flurryCallQueue.splice(0, 1)[0]; this.executeNativeCall(adapterCall); return \); }) (); { } (function () {
var content = 'interstitialinterstitial';
var compiled = Hogan.compile(document.body.innerHTML); var rendered = compiled.render(JSON.parse(content)); document.body.innerHTML = rendered; 
var compiled=Hogan.compile(document.body.innerHTML);var rendered=compiled.render(JSON.parse(content));document.body.innerHTML=rendered;
if(window.mraid){window.mraid.useCustomClose(true);}; 
var compiled = Hogan.compile(document.body.innerHTML); var rendered = compiled.render(JSON.parse(content)); document.body.innerHTML = rendered; 
if(window.mraid) {window.mraid.stateChange(window.mraid.EVENTS.DEFAULT);}}
\end{lstlisting}
} & 4.96 \\ \hline
{\begin{lstlisting}[frame=none,aboveskip=0mm,belowskip=0mm,numbers=none,language=JavaScript,breaklines=true]
document.getElementById('VponVideo').play();
\end{lstlisting}
    } & 4.96 \\ \hline
{\begin{lstlisting}[language=JavaScript,frame=none,aboveskip=0mm,belowskip=0mm,numbers=none,breaklines=true]
function actionClicked(t, u) { var r = prompt('showToast' + JSON.stringify({ method: 'showToast', params: (u ? [t, u] : [t]) })); if (r && typeof r === 'string') { return JSON.parse(r).result; } }; function noTapHighlight() { var l = document.getElementsByTagName('*'); for (var i = 0; i < l.length; i++) { l[i].style.webkitTapHighlightColor = 'rgba(0,0,0,0)'; } }; noTapHighlight();
\end{lstlisting}} & 2.48 \\ \bottomrule
        \end{tabular}
        \caption{Frequent resolved JavaScript code in Malware}
        \label{table:frequent-js-malware}
    % \end{adjustbox}
\end{table*}
