# Supplementary material for: A Large Scale Analysis of Android-Web Hybridization
Source: arXiv:2008.01725 source file (2020-08-05)
Supplement: Supplementary file 2 [file appendixSmaliJS.tex]

%!TEX root = ../Paper.tex
\begin{lstlisting}[float=*,language=Smali,label={listing:smali-dataflow-android-js-appendix},caption={Smali listing called from \emph{onPageFinished() in Liberty Education App}},float=tb]
.method public process()Ljava/lang/Void;
....
iget-object v0, p0, 
Lcom/smaato/soma/bannerutilities/AbstractBannerPackage$InternalWebViewClient$2;->
val$viewFinished:Landroid/webkit/WebView;

const-string v1, #JavaScript string
invoke-virtual {v0, v1}, Landroid/webkit/WebView;->loadUrl(Ljava/lang/String;)V
...
.end method
\end{lstlisting}

\begin{lstlisting}[float=*,language=smali,label={listing:obfuscation-adlocus-appendix},caption={Obfuscation in Library Code-AdLocus},belowskip=0.8\baselineskip,float=tb]
.class public Lcom/adlocus/adapters/AdLocusAdapter;
.super Ljava/lang/Object;
# annotations
.annotation system Ldalvik/annotation/MemberClasses;
    value = {
        Lcom/adlocus/adapters/AdLocusAdapter$a;,
        Lcom/adlocus/adapters/AdLocusAdapter$MyJavascriptInterface;
    }
.end annotation
# instance fields
.field protected final a:Ljava/lang/ref/WeakReference;

.field private b:Landroid/webkit/WebView;
# direct methods
.method public constructor <init>(Lcom/adlocus/AdLocusLayout;)V
...
.end method
.method static synthetic a(Lcom/adlocus/adapters/AdLocusAdapter;)Landroid/webkit/WebView;
...
.end method
.method private a(Lcom/adlocus/AdLocusLayout;)V
    ...
.end method
# virtual methods
.method public a()V
    ...
.end method
.method public b()V
    ...
.end method
.method public c()V
...
.end method
\end{lstlisting}
