# Supplementary material for: A Large Scale Analysis of Android-Web Hybridization
Source: arXiv:2008.01725 source file (2020-08-05)
Supplement: Supplementary file 3 [file appendixSmaliUrl.tex]

%!TEX root = ../Paper.tex

\begin{lstlisting}[float=*,language=Smali, belowskip=-0.8 \baselineskip, caption=WebViewActivity class in com.zipperlockscreenyellow (simplified), label={listing:zipperl-lock-code}, float=htb, escapeinside={*}{*}]
*\label{lst:zipperlockscreenyellow:line_1}* .method public killWebView()V
*\label{lst:zipperlockscreenyellow:line_2}*    [...]
*\label{lst:zipperlockscreenyellow:line_3}*    invoke-virtual {v0}, Landroid/webkit/WebView;->removeAllViews()V
*\label{lst:zipperlockscreenyellow:line_4}*    [...]
*\label{lst:zipperlockscreenyellow:line_5}*    invoke-virtual {v0}, Landroid/webkit/WebView;->clearHistory()V
*\label{lst:zipperlockscreenyellow:line_6}*    [...]
*\label{lst:zipperlockscreenyellow:line_7}*    invoke-virtual {v0, v1}, Landroid/webkit/WebView;->clearCache(Z)V
*\label{lst:zipperlockscreenyellow:line_8}*    [...]
*\label{lst:zipperlockscreenyellow:line_9}*    const-string v1, "about:blank"
*\label{lst:zipperlockscreenyellow:line_10}*    invoke-virtual {v0, v1}, Landroid/webkit/WebView;->loadUrl(Ljava/lang/String;)V
*\label{lst:zipperlockscreenyellow:line_11}*    [...]
*\label{lst:zipperlockscreenyellow:line_12}*    return-void
*\label{lst:zipperlockscreenyellow:line_13}*.end method
\end{lstlisting}

\begin{lstlisting}[float=*,language=Smali, belowskip=-0.8 \baselineskip, caption=The vulnerable method in the EndingScene app (simplified), label={listing:EndingSceneVulnerability}, float=htb, escapeinside={*}{*}]
*\label{lst:vuln:spot_1}*.method protected onCreate(Landroid/os/Bundle;)V
*\label{lst:vuln:spot_2}*
*\label{lst:vuln:spot_3}*    # Setting up the WebView object and enabling JavaScript
*\label{lst:vuln:spot_4}*    [...]
*\label{lst:vuln:spot_5}*  
*\label{lst:vuln:spot_6}*    # Call to loadURL    
*\label{lst:vuln:spot_7}*     iget-object v3, p0, Lcom/endingscene/www/endingscene/MainActivity;->myWebView: Landroid/webkit/WebView;
*\label{lst:vuln:spot_8}*     const-string v4, "http://www.endingscene.com"
*\label{lst:vuln:spot_9}*     invoke-virtual {v3, v4}, Landroid/webkit/WebView;->loadUrl(Ljava/lang/String;)V
*\label{lst:vuln:spot_10}*    
*\label{lst:vuln:spot_11}*    [...]
*\label{lst:vuln:spot_12}*
.end method
\end{lstlisting}
