# Supplementary material for: A Large Scale Analysis of Android-Web Hybridization
Source: arXiv:2008.01725 source file (2020-08-05)
Supplement: Supplementary file 4 [file appendix.tex]

%!TEX root = ../Paper.tex
\begin{lstlisting}[language=python, label={listing:pythonExample}, escapeinside={@}{@}]
from mitmproxy import http

responseBody = b'\
<b>Attackers page:</b>\
<br>\
Username: <input type=\"text\"><br>\
Password: <input type=\"text\"><br>\
'

def request(flow: http.HTTPFlow) -> None:
    if flow.request.pretty_url == "http://www.endingscene.com/":
        flow.response = http.HTTPResponse.make(
            200,  # status code
            responseBody,  # content
            {"Content-Type": "text/html"}  # headers
        )
\end{lstlisting}
